# Supplementary material for: A unified treatment of derivative discontinuity, delocalization and static correlation effects in density functional calculations
Source: arXiv:1710.08973 source file (2018-03-07)
Supplement: Supplementary file 1 [file supplemental.pdf]

## Supplemental Material

### A. Computational settings

$*$ **DMM solver** Following [1], the basis for atomic spin-orbitals $\{|i = m, s\rangle\}$ ($m = -1, \ldots, l$, $s = \alpha, \beta$) was chosen to be real orbitals with angular dependence

$$\Theta(\theta)\Phi(\phi) = \begin{cases} \sqrt{2}\Im Y_{l|m|}(\theta,\phi), & -l \le m < 0 \\ Y_{l0}(\theta,\phi), & m = 0 \\ \sqrt{2}\Re Y_{lm}(\theta,\phi), & 0 < m \le l, \end{cases} \tag{S1}$$

i.e. real-valued spherical harmonics. Since spin-orbit effects are not considered in this work, the presentation of our approach can be simplified such that all the involved quantities in Eq. (1), including the one-body on-site density matrix $\mathbf{n}$, the multi-body density matrix $\mathbb{D}$, Coulomb $\mathbb{V}_{\rm ee}$ and occupancy $\mathbb{N}_{ij}$ matrices, become real. The semidefinite programming problem was solved using the serial version of the CSDP code [2].

$*$ **Density functional calculations** All DFT calculations were carried out using the VASP package [3, 4] with the Perdew-Becke-Ernzerhof (PBE) formulation of the generalized gradient approximation (GGA) exchange-correlation functional [5], projector augmented wave (PAW) potentials [6], and energy cutoff of 450 eV. The volume and shape of the unit cells are fixed at their experimental values.

The tetragonal primitive cell of $KCuF_3$ with type-'a' stacking (space group $I4/mcm$) containing two formula units with a $8\times8\times8$ mesh for $K$-point sampling was used in non-magnetic calculations for the paramagnetic (PM) phase, and a doubled cell with a $8\times8\times4$ $K$-mesh was used for the type-A antiferromagnetic (AF) configuration. LDA+$U$ [7]. We used $J$=0.9 eV and $U$=9 (7) eV for GGA+DMM (GGA+$U$) calculations unless otherwise noted (see discussions below).

### B. DMM further examples [FZ] [FZ : added new section]

A few examples are given in Tables S1,S2 to illustrate how DMM incorporates correlation. Note that while the obtained energy $E_{\rm ee}^{\rm DMM}$ is unique, the many-body density matrix $\mathbb{D}$ that minimizes Eq. (2) may not always be unique. Only one $\mathbb{D}$ is given in the tables.

When the occupancy matrix $\mathbf{n}$ is idempotent (eigenvalues being 0 or 1), the system under consideration is described by a single reference/determinant, and there is no correlation. As a result, DMM energy $E_{\rm ee}^{\rm DMM}$ and the mean-field $E_{\rm ee}^{\rm MF}$ adopted in DFT+$U$ agree. The coincidence vanishes when the eigenvalues of $\mathbf{n}$ become fractional: DFT+$U$ penalizes such $\mathbf{n}$ while $E_{\rm ee}^{\rm DMM}$ remains low by incorporating static correlation, e.g. in $\mathbf{n} = {\rm diag}(\frac{1}{2}, \frac{1}{2})$ for $s$ or ${\rm diag}(\frac{1}{2}, \frac{1}{2}, 0, 0, 0, 0)$ for $p$-electrons.

| $\mathbf{n}$ | $E_{\rm ee}^{\rm DMM}$ | $\mathbb{D}$ | $E_{\rm ee}^{\rm MF}$ | $E_{\rm ee}^{\rm ps}$ | $\mathbf{\Psi}$ |
|---|---|---|---|---|---|
| ${\rm diag}(0,0)$ | 0 | $\lvert\rangle\langle\rvert$ | 0 | 0 | $\lvert\rangle$ |
| ${\rm diag}(1,0)$ | 0 | $\lvert\uparrow\rangle\langle\uparrow\rvert$ | 0 | 0 | $\lvert\uparrow\rangle$ |
| ${\rm diag}(0,1)$ | 0 | $\lvert\downarrow\rangle\langle\downarrow\rvert$ | 0 | 0 | $\lvert\downarrow\rangle$ |
| ${\rm diag}(1,1)$ | $U$ | $\lvert\uparrow\downarrow\rangle\langle\uparrow\downarrow\rvert$ | $U$ | $U$ | $\lvert\uparrow\downarrow\rangle$ |
| ${\rm diag}(\frac{1}{2},\frac{1}{2})$ | 0 | $(\lvert\uparrow\rangle\langle\uparrow\rvert + \lvert\downarrow\rangle\langle\downarrow\rvert)/2$ | $U/4$ | $U/2$ | $(\lvert\rangle + \lvert\uparrow\downarrow\rangle)/\sqrt{2}$ |
| $\begin{pmatrix} 0.6 & 0 \\ 0 & 0.7 \end{pmatrix}$ | $0.3U$ | $0.3\lvert\uparrow\rangle\langle\uparrow\rvert + 0.4\lvert\downarrow\rangle\langle\downarrow\rvert + 0.3\lvert\uparrow\downarrow\rangle\langle\uparrow\downarrow\rvert$ | $0.42U$ | $0.6U$ | $\sqrt{0.3}\lvert\rangle + \sqrt{0.1}\lvert\downarrow\rangle + \sqrt{0.6}\lvert\uparrow\downarrow\rangle$ |
| $\begin{pmatrix} 0.6 & 0.2 \\ 0.2 & 0.7 \end{pmatrix}$ | $0.3U$ | $0.3\lvert\uparrow\rangle\langle\uparrow\rvert + 0.4\lvert\downarrow\rangle\langle\downarrow\rvert + 0.3\lvert\uparrow\downarrow\rangle\langle\uparrow\downarrow\rvert$ $+0.2\lvert\uparrow\rangle\langle\downarrow\rvert + 0.2\lvert\downarrow\rangle\langle\uparrow\rvert$ | $0.38U$ | $0.444U$ | $0.379\lvert\rangle + 0.395\lvert\uparrow\rangle + 0.506\lvert\downarrow\rangle$ $+0.666\lvert\uparrow\downarrow\rangle$ |

TABLE S1. Examples for $s$-electrons ($l = 0$): comparison of DMM (together the density matrix $\mathbb{D}$ that minimizes $E_{\rm ee}^{\rm DMM}$) with the mean-field $E_{\rm ee}^{\rm MF}$ adopted in DFT+$U$ and the pure-state formalism in Eq. (3) (together with the pure state $\mathbf{\Psi}$).

Another way to observe the effects of correlation is through comparison of DMM with the pure-state formalism $E_{\rm ee}^{\rm ps}$ in Eq. (3). As explained in the main text, the search space of DMM is larger than idempotent $\mathbb{D}$ in the latter, leading to more correlation and lower energy ($E_{\rm ee}^{\rm DMM} \le E_{\rm ee}^{\rm ps}$) in DMM, as can be seen from the same examples $\mathbf{n} = {\rm diag}(\frac{1}{2}, \frac{1}{2})$ or ${\rm diag}(\frac{1}{2}, \frac{1}{2}, 0, 0, 0, 0)$. It is noteworthy that in the highly fractional case of $\mathbf{n} = {\rm diag}(\frac{1}{2}, \frac{1}{2}, \frac{1}{2}, \frac{1}{2}, \frac{1}{2}, \frac{1}{2})$, the ground

state $\mathbf{\Psi} = (|\uparrow p_x p_y p_z\rangle + |\downarrow p_x p_y p_z\rangle)/\sqrt{2}$ is inherently multi-determinantal with lower energy $E_{\rm ee}^{\rm ps}$ than the mean-field DFT+$U$. $E_{\rm ee}^{\rm ps}$ may also be higher than $E_{\rm ee}^{\rm MF}$ due to the idempotent $\mathbb{D}$ constraint, e.g. in $\mathbf{n} = {\rm diag}(\frac{1}{2}, \frac{1}{2})$.

| $\mathbf{n}$ | $E_{\rm ee}^{\rm DMM}$ | $\mathbb{D}$ | $E_{\rm ee}^{\rm MF}$ | $E_{\rm ee}^{\rm ps}$ | $\mathbf{\Psi}$ |
|---|---|---|---|---|---|
| ${\rm diag}(1,1,1,0,0,0)$ | $3U-3J$ | $\mathbf{\Psi}\mathbf{\Psi}^\dagger$ | $3U-3J$ | $3U-3J$ | $|\uparrow p_x p_y p_z\rangle$ |
| ${\rm diag}(\frac{1}{2},\frac{1}{2},\frac{1}{2},\frac{1}{2},\frac{1}{2},\frac{1}{2})$ | $3U-3J$ | $(|\uparrow p_x p_y p_z\rangle\langle\uparrow p_x p_y p_z| + |\downarrow p_x p_y p_z\rangle\langle\downarrow p_x p_y p_z|)/2$ | $\frac{15}{4}U-\frac{3}{2}J$ | $3U-3J$ | $(|\uparrow p_x p_y p_z\rangle + |\downarrow p_x p_y p_z\rangle)/\sqrt{2}$ |
| ${\rm diag}(1,1,0,1,0,0)$ | $3U-\frac{3}{5}J$ | $\mathbf{\Psi}\mathbf{\Psi}^\dagger$ | $3U-\frac{3}{5}J$ | $3U-\frac{3}{5}J$ | $|\uparrow p_x p_y \downarrow p_x\rangle$ |
| ${\rm diag}(1,1,0,0,0,1)$ | $3U-\frac{9}{5}J$ | $\mathbf{\Psi}\mathbf{\Psi}^\dagger$ | $3U-\frac{9}{5}J$ | $3U-\frac{9}{5}J$ | $|\uparrow p_x p_y \downarrow p_z\rangle$ |
| ${\rm diag}(\frac{1}{2},\frac{1}{2},\frac{1}{2},0,0,0)$ | $\frac{1}{2}U-\frac{1}{2}J$ | $(|\uparrow p_x\rangle\langle\uparrow p_x| + |\uparrow p_y\rangle\langle\uparrow p_y| + |\uparrow p_z\rangle\langle\uparrow p_z| + |\uparrow p_x p_y\rangle\langle\uparrow p_x p_y| + |\uparrow p_x p_z\rangle\langle\uparrow p_x p_z| + |\uparrow p_y p_z\rangle\langle\uparrow p_y p_z|)/6$ | $\frac{3}{4}U-\frac{3}{4}J$ | $\frac{1}{2}U-\frac{1}{2}J$ | $(|\uparrow p_x\rangle + |\uparrow p_y p_z\rangle)/\sqrt{2}$ |
| ${\rm diag}(\frac{1}{2},\frac{1}{2},0,0,0,0)$ | $0$ | $(|\uparrow p_x\rangle\langle\uparrow p_x| + |\uparrow p_y\rangle\langle\uparrow p_y|)/2$ | $\frac{1}{4}U-\frac{1}{4}J$ | $\frac{1}{2}U-\frac{1}{2}J$ | $(|\rangle + |\uparrow p_y p_z\rangle)/\sqrt{2}$ |

TABLE S2. Examples for $p$-electrons ($l=1$): DMM energy for different $\mathbf{n} = {\rm diag}(n_{px\alpha}, n_{py\alpha}, n_{pz\alpha}, n_{px\beta}, n_{py\beta}, n_{pz\beta})$.

## C. $U$-dependence

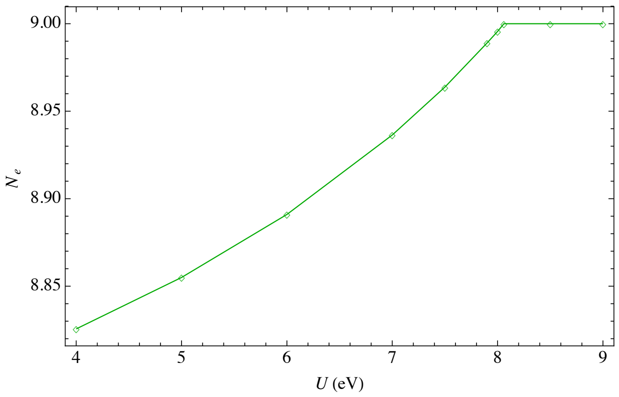


FIG. S1. GGA+DMM prediction of $N_{\rm e}$ in $KCuF_3$ vs. $U$ with fixed $J$=0.9 eV.

The dependence of the number of $3d$-electrons $N_{\rm e}$ in $KCuF_3$ on the $U$ parameter according to GGA+DMM is depicted in Fig. S1. Below the critical value $U_{\rm crit}$=8.06 eV, the derivative discontinuity is not enough to overcome the kinetic energy, and consequently GGA+DMM predicts strictly speaking a metallic electronic structure while $N_{\rm e}$ remains a fractional number close to but smaller than $z_{\rm e} = 9$. Above $U_{\rm crit}$, a metal-insulator transition occurs, pinning $N_{\rm e}$ to $z_{\rm e} = 9$ accompanied by a band gap of $\mathcal{D}_{\rm xc} = U - xJ$. This is accomplished by applying in addition the opposing crystal potential (OCP) method developed previously [8]. Other than the band gap, the $U$-dependence of the potential energy surface is negligibly small above $U_{\rm crit}$. In this work, we report GGA+DMM results for the insulating state above $U_{\rm crit}$. Note that Ref. [9] applied $J$=0.9 eV and a smaller $U$=7 eV for GGA+DMFT calculations.

## D. $J$-dependence and more detailed results on $KCuF_3$

Fig. S2 shows the $J$-dependence of the stabilization energy. With small $J$, GGA+DMM tend to under-polarize, leading to very weak stabilization of JT distortions. Increase of $J$ to physical values around 1 eV leads to much more substantial polarization and stabilization. The sensitivity to the $J$ value lies in the required corrections to the substantial aspherical self-interaction errors proportional to $J$ [1] due to the symmetry breaking Jahn-Teller distortion.

| | PM $\delta_{\rm opt}$ ($\Delta E_{\rm JT}$) | AF $\delta_{\rm opt}$ ($\Delta E_{\rm JT}$) | $\Delta E_{\rm mag}$ |
|---|---|---|---|
| GGA | 3.2% (-10) | 3.5% (-27) | 38 |
| GGA+$U$ | 4.2% (-85) | 4.0% (-160) | 912 |
| GGA+DMM | 4.0% (-62) | 4.1% (-74) | 18 |

TABLE S3. Optimal Jahn-Teller distortion $\delta_{\rm opt}$ and stabilization energy in meV $\Delta E_{\rm JT} = E(\delta_{\rm opt}) - E(\delta = 0)$ for different magnetic configurations. The PM-AF energy difference $\Delta E_{\rm mag} = E(\delta, {\rm PM}) - E(\delta, {\rm AF})$ at experimental $\delta$=4.4% is also given.

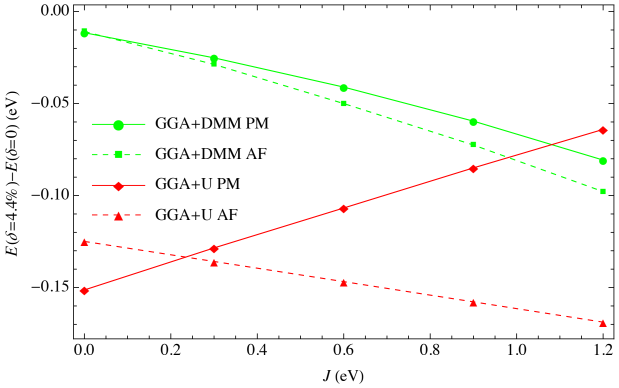


FIG. S2. Dependence on the $J$ parameter of the energy difference $E(\delta = 4.4\%) - E(\delta = 0)$ per $KCuF_3$ in different magnetic configurations using GGA+$U$, and GGA+DMM with fixed $U$=7 eV.


[1] F. Zhou and V. Ozolins, Phys. Rev. B **80**, 125127 (2009).
[2] B. Borchers, Optim. Methods Softw. **11**, 613 (1999).
[3] G. Kresse and J. Furthmuller, Phys. Rev. B **54**, 11169 (1996).
[4] G. Kresse and D. Joubert, Phys. Rev. B **59**, 1758 (1999).
[5] J. P. Perdew, K. Burke, and M. Ernzerhof, Phys. Rev. Lett. **77**, 3865 (1996).
[6] P. E. Blochl, Phys. Rev. B **50**, 17953 (1994).
[7] N. Binggeli and M. Altarelli, Phys. Rev. B **70**, 085117 (2004).
[8] F. Zhou and D. Åberg, Phys. Rev. B **93**, 085123 (2016).
[9] I. Leonov, N. Binggeli, D. Korotin, V. I. Anisimov, N. Stojic, and D. Vollhardt, Phys. Rev. Lett. **101**, 096405 (2008).
